# Supplementary material for: The OpenPicoAmp : an open-source planar lipid bilayer amplifier for hands-on learning of neuroscience
Source: arXiv:1403.7439 ancillary file (2014-12-14)

# Implementation of the amplifier

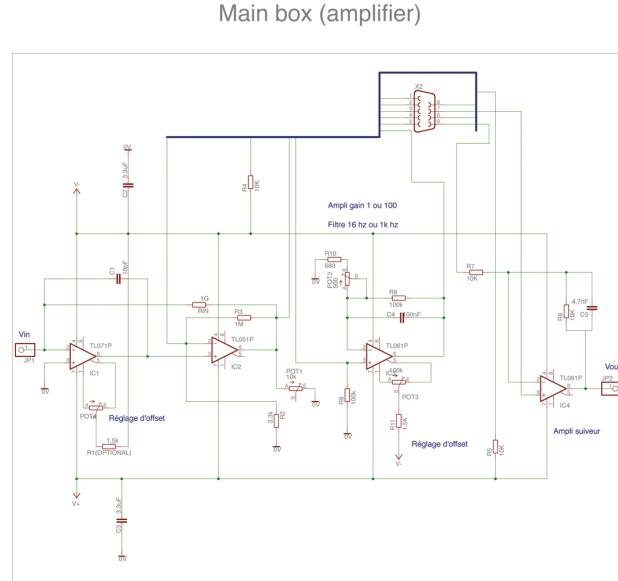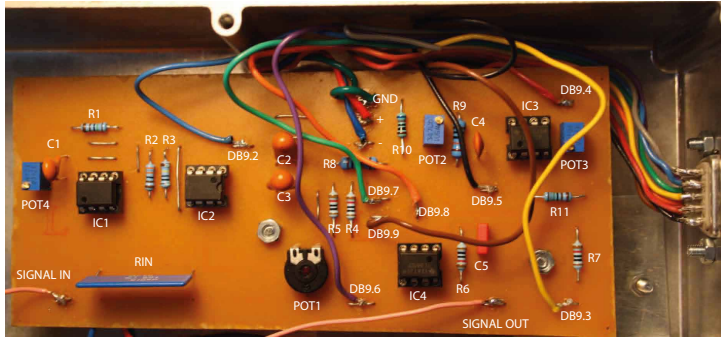

Figure 7: Circuit schematics and implementation of the amplifier in the main box. The blue line represents a bus. The wiring can be followed by opening the schematic file (S2.OpenPicoAmp.sch) and using the "show" tool in the Eagle software.

The OpenPicoAmp can be implemented by following these steps :

- order or print the board circuit (PCB) according the proposed layout (given at end of this document).
- individual components have to soldered to the PCB according to the board layout (fig. 7) contained in the file S1 (S1.OpenPicoAmpBoard.brd). Respect carefully the polarity of the capacitors C2 and C3.
- the main box needs to be drilled to install the following : two BNC connectors to the recording chamber, one BNC connector for the input signal, one BNC connector for the output signal, a two positions power switch and a DB9 connector for the remote control.

Remote control (gain & offset)

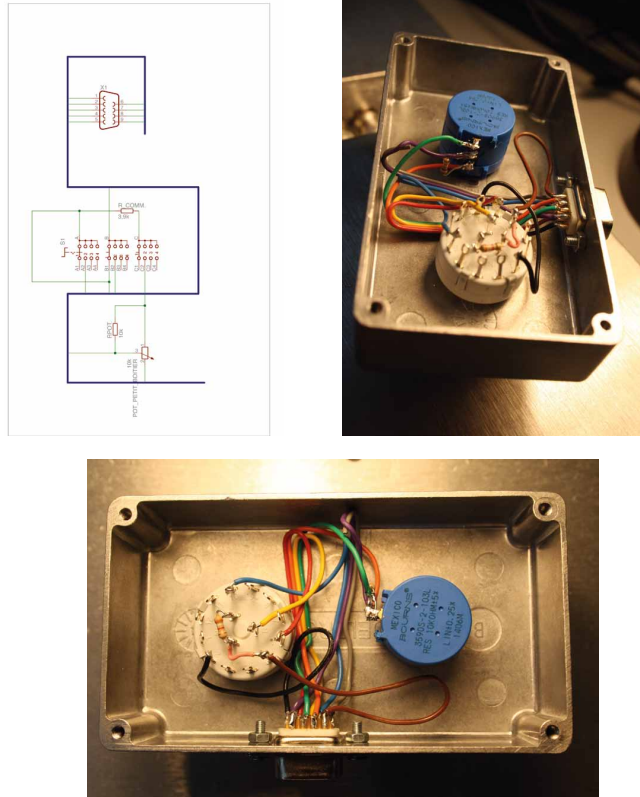

Figure 8: Circuit schematics and implementation of the remote control. The blue line represents a bus. The wiring can be followed by opening the schematic file (S2\_OpenPicoAmp.sch) and using the "show" tool in the Eagle software.

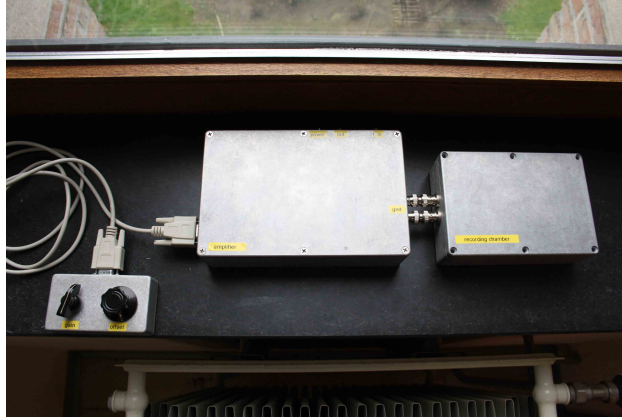

Figure 9: The complete setup including the amplifier, the recording chamber and the remote control.

- the PCB board should be installed in the enclosure of the main box and connected to the other components, including the two 6V battery holders (fig. 1).
- the next step is to make the remote control, which contains a  $10\text{ k}\Omega$  potentiometer, a 3 poles 4 positions rotary switch, a  $10\text{ k}\Omega$  resistor, a  $3.9\text{ k}\Omega$  resistor and a DB9 connector. The corresponding schematics and the proposed implementation is shown on fig. 8.
- the recording chamber needs to be drilled to install the two BNC connectors.
- connect the remote control to the amplifier with a RS232 DB9 cable and connect the main box to the recording chamber using the two BNC-BNC adapters (fig. 9).
- switch the amplifier on.
- on the first use, the OpenPicoAmp needs to be calibrated by adjusting the potentiometers POT1, POT2, POT3 and POT4. For that a  $50\text{ }\Omega$  BNC terminator should be connected to the input of the amplifier, the model circuit (composed of a  $1\text{ G}\Omega$  resistance with a  $220\text{ pF}$  capacitor in parallel ) should be connected to the BNC in the recording chamber (lid closed) and the output of the amplifier should be connected to an oscilloscope.
- the potentiometer of the remote control should be precisely halfway, with  $0\text{V}$  at its output.
- with the amplifier set on gain  $1\text{ mV/pA}$ , use POT4 to adjust the output at  $0\text{V}$ .
- with the amplifier set on gain  $100\text{ mV/pA}$ , use POT3 to adjust the output at  $0\text{V}$ .
- remove the  $50\text{ }\Omega$  BNC terminator and connect the input of the amplifier to an ajustable DC source.
- with the amplifier set on gain  $100\text{ mV/pA}$  and a constant voltage of  $10\text{ mV}$  at the input of the amplifier, use POT2 to adjust the output at  $1\text{ V}$ .
- connect the input of the amplifier to a function generator delivering a  $500\text{ Hz}$   $10\text{ mV}$  peak to peak triangular signal.
- with the amplifier set on gain  $1\text{ mV/pA}$ , use POT1 to adjust the shape of the signal so it appears as square as possible.

OPENPICOAMP

| Components                                   | Farnell       |           | Qty | Description                                    | Cost  | Tag                  |
|----------------------------------------------|---------------|-----------|-----|------------------------------------------------|-------|----------------------|
|                                              | Cost/Unit (€) | Part #    |     |                                                |       |                      |
| STMICROELECTRONICS TL071CN                   | 0.94          | 1094351   | 1   | 1 IC, OP AMP, JFET                             | 0.94  | IC1                  |
| TEXAS INSTRUMENTS TL061CP                    | 0.62          | 1103000   | 3   | OP AMP, SINGLE, 1MHZ, MICROPOWER, 8DIP         | 1.86  | IC2, IC3, IC4        |
| VISHAY SPRAGUE 561R10TC C Q10                | 0.77          | 1702661   | 1   | 1 CERAMIC DISC CAPACITOR 10PF                  | 0.77  | C1                   |
| OHMITE SM102031007FE.                        | 2.27          | 1159363   | 1   | 1 RESISTOR, THICK FILM, 1GOHM, 1.5W, 1%        | 2.27  | Rin                  |
| VISHAY BC COMPONENTS - MRS25000C1501FCT00    | 0.06          | 9465359   | 2   | 2 RESISTOR, THIN FILM, 1.5K, 0.6W, 1%          | 0.11  | R1 (optional), R11   |
| VISHAY BC COMPONENTS - MRS25000C3301FCT00    | 0.06          | 9467823   | 1   | 1 RESISTOR, 3K3, 1%, 0.6W, AXIAL               | 0.06  | R2                   |
| VISHAY BC COMPONENTS - MRS25000C1004FCT00    | 0.08          | 9465499   | 1   | 1 RESISTOR, THIN FILM, 1W, 0.6W, 1%            | 0.08  | R3                   |
| VISHAY BC COMPONENTS - MRS25000C1002FCT00    | 0.09          | 9463976   | 5   | 5 RESISTOR, THIN FILM, 10K, 0.6W, 1%           | 0.46  | R4, R5, R6, R7, RPOT |
| MULTICOMP - MF50 100K                        | 0.02          | 9339795   | 2   | 2 RESISTOR, 100K, 0.5W, 1%                     | 0.04  | R8, R9               |
| MULTICOMP - MCMF006FF6800A50                 | 0.01          | 2401749   | 1   | 1 RESISTOR, METAL FILM, 680 OHM, 1%, AXIAL     | 0.01  | R10                  |
| MULTICOMP - MF50 3K9                         | 0.04          | 9340521   | 1   | 1 RESISTOR, 0.5W 1% 3K9                        | 0.04  | R_COMM               |
| MULTICOMP - CB1V335M2BCB                     | 0.55          | 9708545   | 2   | 2 CAP TANT, 33UF, 35V, RAD                     | 1.1   | C2, C3               |
| MULTICOMP MCFYU6104Z6                        | 0.14          | 9411887   | 1   | 1 CAP, CERAMIC, 0.1UF, 50V, Y5V, RAD           | 0.14  | C4                   |
| MURATA DE1E3KX472MA4BL01                     | 0.6           | 1515825   | 1   | 1 CAPACITOR, SAFETY, 4.7NF, 250V, 20%          | 0.6   | C5                   |
| BI TECHNOLOGIES/TT ELECTRONICS - 38PKABR10KL | 0.74          | 1417145   | 1   | 1 TRIMMER, POTENTIOMETER 10KOHM 1TURN PCB      | 0.74  | POT1                 |
| BOURNS 3266W-1-501LF                         | 3.59          | 9352740   | 1   | 1 TRIMMER, 15 TURN 500R                        | 3.59  | POT2                 |
| BOURNS 3266W-1-104LF                         | 3             | 9352660   | 2   | 2 POT, TRIMMER, 100K, 12 TURN, 3 PIN           | 6     | POT3, POT4           |
| TE CONNECTIVITY / GREENPAR 1-1337451-0       | 4.12          | 110562661 | 4   | 4 RFCOAXIAL, BNC, STRAIGHT JACK, 50OHM         | 16.48 |                      |
| NORCOMP 170-009-103L001                      | 0.83          | 2294224   | 1   | 1 D-SUB, PLUG, SOLDFR, STRAIGHT, 9WAY          | 0.83  | X1, X2               |
| NORCOMP 171-009-203L001                      | 0.76          | 2294225   | 1   | 1 D-SUB, RECEPTACLE, SOLDFR, 9WAY              | 0.76  |                      |
| LORLIN CK1026                                | 2.05          | 1123704   | 1   | 1 SWITCH, 3POLE, 4POS, 0.15A, 250V, SOLDER     | 2.05  | S1                   |
| NEUTRIK NBR75FG                              | 7.46          | 4709603   | 2   | 2 BULKHEAD ADAPTER, BNC JACK-BNC JACK          | 14.92 |                      |
| TE CONNECTIVITY / GREENPAR 1-1478043-0       | 16.6          | 1056275   | 2   | 2 ADAPTER, BNC PLUG, BNC PLUG, 75OHM           | 33.2  |                      |
| BOURNS - 3590S-2-103L                        | 16.15         | 1612611   | 1   | 1 POTENTIOMETER 10KR 2W                        | 16.15 | POT_PETIT_BOTTIER    |
| KEYSTONE - 2478                              | 1.96          | 1650685   | 2   | 2 BATTERY HOLDER, LEADED, 4 X AA               | 3.92  |                      |
| TE CONNECTIVITY - 808-AG11D-LF               | 2.17          | 1077303   | 4   | 4 DIP SOCKET, 8POS, THROUGH HOLE               | 8.68  |                      |
| DELTRON 459-0070                             | 25.13         | 279110    | 1   | 1 cast aluminium enclosure (amplifier)         | 25.13 |                      |
| DELTRON 459-0050                             | 19.95         | 279092    | 1   | 1 cast aluminium enclosure (recording chamber) | 19.95 |                      |
| DELTRON 459-0020                             | 10.2          | 525613    | 1   | 1 cast aluminium enclosure (remote control)    | 10.2  |                      |

Total (EUR)  
160.87

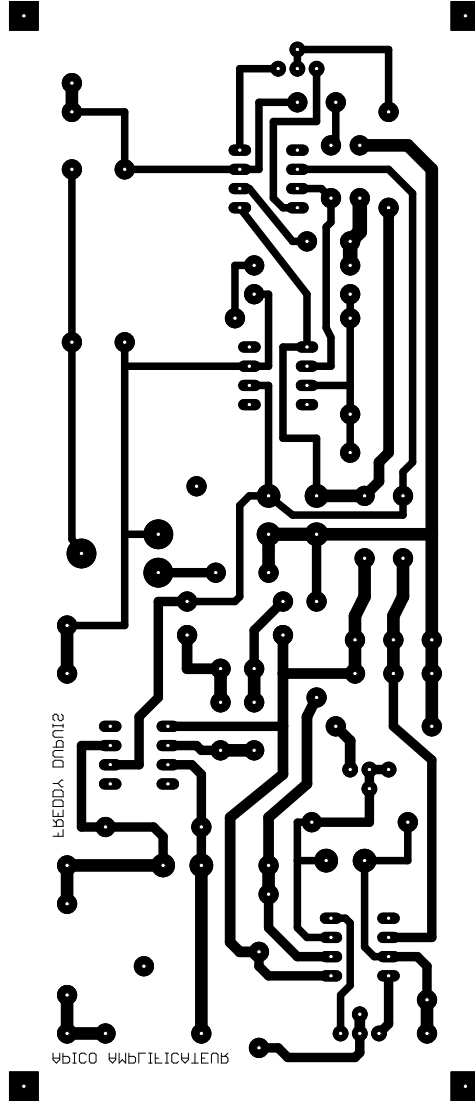

Supplement: Supplementary file 1 [file S3_OpenPicoAmp_implementation.pdf]
