# Supplementary material for: The OpenPicoAmp : an open-source planar lipid bilayer amplifier for hands-on learning of neuroscience
Source: arXiv:1403.7439 ancillary file (2014-12-14)
Supplement: Supplementary file 4 [file S8_SurveyBLM.pdf]

Please fill **BEFORE** the lab session

**Equivalent circuit of the passive cell membrane**

The intensity of the current flowing through the test circuit is higher when it is submitted to a the AC voltage compared to the DC voltage ? T F  
☐ ☐

The capacitive current is zero when the applied voltage is constant. ☐ ☐

The total current is purely resistive when the applied voltage is constant. ☐ ☐

**Membrane capacitance of the planar lipid bilayer**

The electric field is constant inside the lipid bilayer and zero outside. T F  
☐ ☐

The capacitance of the bilayer is a function of its radius. ☐ ☐

The observed capacitance decreases during the lipid bilayer formation. ☐ ☐

**Membrane resistance of the planar lipid bilayer**

Lipids are a good insulator. T F  
☐ ☐

The bilayer resistance changes in asymmetric ionic conditions compared to its value in symmetric ionic conditions. ☐ ☐

Lipid resistivity is a function of the thickness of the bilayer. ☐ ☐

**Ionic channels**

Ionic channels formed by gramicidin molecules behave as ohmic conductors. T F  
☐ ☐

The total conductance is obtained by multiplying the total number of channels by the unitary conductance and by the open probability. ☐ ☐

Unitary currents are zero at a 0 mV holding potential in asymmetric ionic conditions. ☐ ☐

Please fill **AFTER** the lab session

**Equivalent circuit of the passive cell membrane**

- |                                                                                                                                               | T                        | F                        |
|-----------------------------------------------------------------------------------------------------------------------------------------------|--------------------------|--------------------------|
| The intensity of the current flowing through the test circuit is higher when it is submitted to a the AC voltage compared to the DC voltage ? | <input type="checkbox"/> | <input type="checkbox"/> |
| The capacitive current is zero when the applied voltage is constant.                                                                          | <input type="checkbox"/> | <input type="checkbox"/> |
| The total current is purely resistive when the applied voltage is constant.                                                                   | <input type="checkbox"/> | <input type="checkbox"/> |

**Membrane capacitance of the planar lipid bilayer**

- |                                                                           | T                        | F                        |
|---------------------------------------------------------------------------|--------------------------|--------------------------|
| The electric field is constant inside the lipid bilayer and zero outside. | <input type="checkbox"/> | <input type="checkbox"/> |
| The capacitance of the bilayer is a function of its radius.               | <input type="checkbox"/> | <input type="checkbox"/> |
| The observed capacitance decreases during the lipid bilayer formation.    | <input type="checkbox"/> | <input type="checkbox"/> |

**Membrane resistance of the planar lipid bilayer**

- |                                                                                                                    | T                        | F                        |
|--------------------------------------------------------------------------------------------------------------------|--------------------------|--------------------------|
| Lipids are a good insulator.                                                                                       | <input type="checkbox"/> | <input type="checkbox"/> |
| The bilayer resistance changes in asymmetric ionic conditions compared to its value in symmetric ionic conditions. | <input type="checkbox"/> | <input type="checkbox"/> |
| Lipid resistivity is a function of the thickness of the bilayer.                                                   | <input type="checkbox"/> | <input type="checkbox"/> |

**Ionic channels**

- |                                                                                                                                       | T                        | F                        |
|---------------------------------------------------------------------------------------------------------------------------------------|--------------------------|--------------------------|
| Ionic channels formed by gramicidin molecules behave as ohmic conductors.                                                             | <input type="checkbox"/> | <input type="checkbox"/> |
| The total conductance is obtained by multiplying the total number of channels by the unitary conductance and by the open probability. | <input type="checkbox"/> | <input type="checkbox"/> |
| Unitary currents are zero at a 0 mV holding potential in asymmetric ionic conditions.                                                 | <input type="checkbox"/> | <input type="checkbox"/> |
